# Supplementary material for: On the Computational Consequences of Cost Function Design in Nonlinear Optimal Control
Source: arXiv:2204.01986 source file (2022-11-18)
Supplement: Supplementary file 1 [file appendix_arxiv.tex]

\subsection{Auxilary Lemmas}

\begin{lemma} \label{lemma:min_phase_rate}
Let the assumptions in Lemma \ref{lemma:growth} hold. Then there exists constants $C_1, C_2,C_3>0$ and such that for each $\epsilon>0$ sufficiently small there exists a continuously differentiable function $W^\epsilon \colon \R^n \to \R^n$ which satisfies for each $(\tilde{\xi},\eta) \in \R^n$ and $u \in \R^q$:
\begin{equation}
    C_1\big(\epsilon\|\tilde{\xi}\|_2^2+ \|\eta\|_2^2\big)\leq W^\epsilon(\tilde{\xi},\eta) \leq C_2\big(\epsilon\| \tilde{\xi}\|+ \|\eta\|_2^2\big) 
\end{equation}
\begin{equation}
    \dot{W}(\tilde{\xi}, \eta,\tilde{u}) \leq -C\big(\| \tilde{\xi}\|_{2}^2 + \|\eta\|_2^2 \big)+ \|\tilde{\xi}_1 \|_2^2 + \|\tilde{u}\|_2^{2}
\end{equation}
\end{lemma}
\begin{proof}
  First, choose the matrix $M$ such that the matrix $F+MH$ is Hurwitz with $F,H$ as in \eqref{eq:matrix_def} (note that this is possible because $(F,H)$ is observable). Then select $P$ such that $(F+MH)^TP + P(F+MH) = - 2I$. Next, let the function $V(\eta)$ be obtained from the converse exponential stability theorem as in the proof of Lemma \ref{lemma:growth}. Without loss we assume that $c_3>2$ (if this is not the case we can re-scale $V$ to $\alpha V$ below for $\alpha>1$ sufficiently large). We then define for each $\epsilon>0$, $W^\epsilon(\tilde{\xi},\eta) = \epsilon \tilde{\xi}^{T}P\tilde{\xi} + V(\eta)$. The time derivative of this function satisfies: 
\begin{align}
\dot{W}^\epsilon(\tilde{\xi},\eta,\tilde{u})&= \tilde{\xi}^T(F^T P +PF)\xi + 2 \tilde{\xi}^TPG\epsilon^{r}\tilde{b}(\tilde{\xi},\eta)\\\nonumber &+ 2 \tilde{\xi}^TPG\tilde{A}(\tilde{\xi},\eta)u + \frac{d}{d\eta}V(\eta)[f_0(\eta) + g_0(\eta)\tilde{\xi}_1] 
\end{align}
Using the definition of $P$ above and $\frac{d}{d\eta} V(\eta)f_0(\eta) < -c_3 \|\eta \|_2^{2}< -2\| \eta\|_2^{2}$ and $\| \frac{d}{d\eta}V(\eta)\|_2 \leq c_4$ as in the proof of Lemma \ref{lemma:growth}, and the growth conditions in Assumption \ref{asm:growth}, in particular, $\epsilon^r \|\tilde{b}(\tilde{\xi},\eta)\|_2 \leq L(\epsilon \|\tilde{\xi}\|_2 +  \epsilon^r\|\eta\|_2)$, from the preceding equation we obtain:
\begin{align*}
    &\dot{W}^\epsilon(\tilde{\xi},\eta,\tilde{u}) \leq -2(\| \tilde{\xi}\|_2^{2} +\|\eta\|_2^2) + 2\epsilon L\|PG\|_2 \|\tilde{\xi}\|_2(\|\tilde{\xi}\|_2 + \| \eta\|_2) \\ \nonumber
    & +C\|PG\|_2 \| \tilde{\xi}\|_2\|u\|_2 + c_4C\|\eta\|_2 \| \tilde{\xi}\|_2 + \tilde{\xi}(H^TL^TP + PLH)\tilde{\xi}\\
    &\leq -2(\| \tilde{\xi}\|_2^{2} + \|\eta\|_2^2) + 2\epsilon L\|PG\|_2 (\|\tilde{\xi}\|_2^2 + \| \eta\|_2\|\tilde{\xi}\|_2) \\ \nonumber
    & +C\|PG\|_2 \| \tilde{\xi}\|_2\|u\|_2 + c_4C\|\eta\|_2 \| \tilde{\xi}_1\|_2 + 2\|PL\|_2\|\tilde{\xi}\|_2\|\tilde{\xi}_1\|_2\\
    &\leq -2(\| \tilde{\xi}\|_2^{2} +  \|\eta\|_2^2) +(\|\tilde{\xi}\|_2^2 +\|\eta\|_2^2) + 3\epsilon L\|PG\|_2 (\|\tilde{\xi}\|_2^2 \\ \nonumber
    & +\|\eta \|_2^2)  +\frac{1}{2}C\|PG\|_2\|u\|_2^2 +  (\frac{1}{2}c_4C  + \|PL\|_2\|)\|\tilde{\xi}_1\|_2^2,
\end{align*}
where in the final step we have repeatedly used the AM-GM inequality. The final expression demonstrates that $\alpha W^\epsilon$ has the desired properties for $\alpha < \min\{\frac{1}{2}C\|PG\|_2,\frac{1}{2}c_4C  + \|PL\|_2\|\}$ and sufficiently small $\epsilon$. 
\end{proof}

\subsection{Performance Bounds}

\subsubsection{Proof of Lemma \ref{lemma:growth}}
\begin{proof}
To provide the performance guarantee we will apply a sub-optimal feedback linearizaing controller of the the form $\tilde u = \tilde{A}^{-1}(\tilde{\xi},\eta)[-\tilde{\epsilon}^r\tilde b(\tilde{\xi}, \eta) + K\tilde{\xi}]$ to the fast-slow representation of the dynamics \eqref{eq:transformed_dyn}, where $K$ is chosen such that for some $M > 0$, $\|\tilde \xi(t)\|_2 \leq M e^{-
\frac{t}{\epsilon}}\|\tilde \xi(0)\|_2$ for all $t \geq 0$. We will  prove the result for the case where the system is not full-state linearizable; the proof for the full-state linearizable case follows by simply ignoring terms related to the zeros in the proof.

Note that, by Assumption \ref{asm:relative_degree}, since the matrix $\bar{A}(\xi,\eta)$ is bounded away from singularity, there exists a constant $\gamma>0$ such that $\|\tilde{A}^{-1}(\tilde \xi,\eta)\| \leq \frac{1}{\gamma}$ holds uniformly. Further note that $\|\tilde{\xi}_1(t)\|_2 \leq \|\tilde \xi(t)\|_2$ for all $t \geq 0$.  We can further bound $\tilde{\epsilon}^{2r}\|\tilde b(\tilde {\xi}, \eta)\|_2^2 = \tilde{\epsilon}^{2r}\|b(S^{-1}(\tilde{\epsilon}) \tilde{ \xi},\eta)\|_2^2 \leq \frac{3}{2}C^2\tilde{\epsilon}^{2r}(\|S^{-1}(\tilde{\epsilon}) \tilde{ \xi}\|_2^2 + \|\eta\|_2^2) \leq \frac{3}{2}C^2\tilde{\epsilon}^{2r}(\frac{1}{\tilde{\epsilon}^{2(r-1)}} \|\tilde{\xi}\|_2^2 + \|\eta\|_2^2) = \frac{3}{2}C^2  ( \epsilon^2\|\tilde{\xi}\|_2^2 +\tilde{\epsilon}^{2r} \|\eta\|_2^2)$ , where we have used Assumption \ref{asm:growth} and $(\|S^{-1}(\tilde{\epsilon})\tilde{\xi}\|_2 + \|\eta \|_2)^2 \leq \frac{3}{2}(\|\tilde{\xi} \|_2^2 + \| \eta\|_2^2)$. Thus, we have:
\begin{align*} 
    \|\tilde{u}(t)\|_2^2 &\leq \| \tilde{A}^{-1}(\tilde{\xi},\eta)\|_2^2 \cdot \bigg( \frac{3}{2}(\epsilon^2\|\tilde{\xi}\|_2^2 + \tilde{\epsilon}^{2r}\|\eta(t)\|_2^2 )\\
    & \ \ \ \ \ \ \ \ \ \ \ \ \ \ \ \  + \|K\|_2^2 \| \tilde{\xi}\|_2^2 \bigg). \\
    &  \leq C_1( \| \tild{\xi}\|_2^2 + \tilde{\epsilon}^{2r}\|\eta(t)\|_2^2)
\end{align*}
for some $C_1>0$ sufficiently large. 

We now try to find a bound on $\|\eta(t)\|_2^2$. As $\dot \eta = f_0(\eta)$ is exponentially stable, by the converse Lyapunov theorem $\exists c_1,c_2,c_3,c_4 > 0$ and $V(\eta)$ a Lyapunov function s.t $\forall \eta$:
\begin{align*}
c_1\|\eta\|_2^2 \leq V(\eta) &\leq c_2\|\eta\|_2^2,\\ \frac{dV(\eta)}{d\eta}f_0(\eta) &\leq - c_3\|\eta\|_2^2,\\ 
\|\frac{dV(\eta)}{d\eta}\|_2 &\leq c_4\|\eta\|_2
\end{align*}
Now consider the time derivative of $V(\eta)$ along the full system dynamics:
\begin{align*}
    \dot V(\eta) &= \frac{dV(\eta)}{d\eta}(f_0(\eta) + g_0(\eta)\tilde{\xi}_1) \\
    &\leq -c_3\|\eta\|_2^2 + \|\frac{dV(\eta)}{d\eta}\|_2\|g_0(\eta)\|_2\|\tilde{\xi}_1\|_2 \\
    &\leq -c_3\|\eta\|_2^2 + c_4\|g_0(\eta)\|_2\|\eta\|_2\|\tilde \xi\|_2 \\
    &\leq (c^2_4Ck-c_2)\|\eta\|^2_2 + \frac{1}{k}\|\tilde \xi\|^2_2 \\
    &\leq (\frac{c^2_4Ck}{c_2}-1)V(\eta) + \frac{1}{k}\|\tilde \xi\|^2_2 = -\tilde c V(\eta) + \frac{1}{k}\|\tilde \xi\|^2_2
\end{align*}
where $k$ s.t $\tilde c = 1-\frac{c^2_4Ck}{c_2} > 0$. If we henceforth choose $\tilde{\epsilon}>0$ to be small enough so that $\tilde{c} -\frac{1}{\tilde{\epsilon}}< \frac{-1}{2\tilde{\epsilon}}$ when we can use the bounds on $V$ to obtain:
\begin{align*}
    V(\eta(t)) &\leq e^{-\tilde ct}V(\eta(0)) + \frac{1}{k}\int_0^t e^{-\tilde c(t-\tau)}\|\tilde \xi(\tau)\|\cdot d\tau \\
    & = \leq e^{-\tilde ct}\bigg(V(\eta(0)) +\frac{M^2}{k}\int_{0}^t e^{ -\frac{1}{ \tilde{\epsilon}}\tau}\|  \tilde{\xi}(0)\|_2^2 d\tau \bigg) \\
    & \leq e^{-\tilde ct}\bigg( V(\eta(0)) +\frac{M^2 \tilde{\epsilon}}{k}\|\tilde{\xi}(0)\|_2^2 \bigg)
\end{align*}
And 
\begin{align*}
    \|\eta(t)\|_2^2 & \leq e^{-\tilde ct}\bigg(\frac{c_2}{c_1}\|\eta(0)\|_2^2 + \frac{M^2 \tilde{\epsilon}}{c_1k}\|\tilde \xi(0)\|_2^2\bigg) \\
    &\leq C_2 e^{-\tilde{c}t} \bigg(\|\eta(0)\|_2^2 + \epsilon \|\tilde{\xi}(0)\|_2^2\bigg)
\end{align*},
for some $C_2>0$ sufficiently large.

Putting these bounds together gives yields:
\begin{align*}
    \tilde{V}_\infty^{\tilde{\epsilon}}(x) &\leq \int_0^\infty \|\tilde{\xi}_1(t)\|_2^2 + \|\tilde{u}(t)\|_2^2 dt \\
    & \leq \|\tilde{\xi}(t)\|_2^2 + C_1(\tilde{\epsilon}^2\|\tilde{\xi}(t)\|_2^2 +\tilde{\epsilon}^{2r}\|\eta (t)\|_2^2) dt \\
    &\leq  \int_{0}^{\infty}\bigg((1+\tilde{\epsilon}^2)M^2e^{\frac{-2}{\tilde{\epsilon}}t}\|\tilde{\xi}(0)\|_2^2\\
    &+ C_1C_2 \tilde{\epsilon}^{2r} e^{-\tilde{c}t}\big( \| \eta(0)\|_2^2 + \tilde{\epsilon}\|\tilde{\xi}(0)\|_2^2\big) \bigg) dt \\
    &\leq C_3\big(\tilde{\epsilon} \|\tilde{\xi}(0)\|_2^2 + \tilde{\epsilon}^{2r}\| \eta(0)\|_2^2\big),
\end{align*}

for some $C_3>0$ sufficiently large. 
\end{proof}

\subsection{Proof of Lemma \ref{lem:growth_finite} }

\newline 
\begin{proof}
We again apply a control of the form
 by $\bar{u}= \tilde{A}^{-1}(\tilde{\xi}(t),\eta(t))[-\tilde{b}(\tilde{\xi}(t),\eta(t)) + K\tilde{\xi}(t)]$ where $K$ is chosen so that $F+GK$ is Hurwitz and chosen so that for some $M>0$ we have $\tilde{\xi}(t) \leq Me^{-\frac{t}{\epsilon}}\|\tilde{\xi}(t)\|$. Next we seek to bound the growth of the zeros under the application of this control law:
\begin{align}
\frac{d}{dt} (\| \eta(t)\|_2^2 )&= 2 \eta(t)^T[f_0(\eta) + g(\eta)\tilde{\xi}] \\
& \leq 2 C\|\eta(t)\|_2^2 + 2C\|\eta(t) \|_2\|\tilde{\xi}(t) \|_2 \\
&\leq 4C\|\eta(t)\|_2^2 + 2C\| \tilde{\xi}(t)\|_2^2\\
&\leq K_1 \left(\|\eta(t)\|_2^2 + \| \tilde{\xi}(t)\|\right) ,
\end{align}
where we have used Assumption \ref{asm:growth} the inequality $a\cdot b \leq \frac{1}{2}(a^2 + b^2)$,
and have chosen $K_1>0$ to be sufficiently large. By the comparison principle the preceding inequality yields:
\begin{align}
\|\eta(t) \|_2^2 &\leq e^{K_1t}\| \eta(0)\| + \int_{0}^{t}  e^{K_1(t-\tau)}\|\tilde{\xi}(\tau)\|_2^2 d\tau \\
&\leq e^{K_1t}\| \eta(0)\| \\
&+ e^{K_1 \bar{T}}\int_{0}^{t}  Me^{-\frac{1}{\epsilon}\tau}\|\tilde{\xi}(0)\|_2^2 d\tau \\
&\leq K_2(\|\eta(0)\|_2^2 + \epsilon \| \xi(0)\|),
\end{align}
where $K_2>0$ is chosen to be sufficiently large. As was done in the proof of Theorem \ref{lemma:growth}, we can obtain a bound for the linearizing controller of the form:
\begin{equation}
    \|\tilde{u}(t)\|_2^2 \leq K_3 (\|\tilde{\xi}(t)\|_2^2 + \tilde{\epsilon}^{2r} \|\eta(t)\|_2^2).
\end{equation}
Thus, we have:
\begin{align*}
\tilde{V}_T^{\tilde{\epsilon}}(\tilde{\xi}(0),\eta(0)) &\leq \int_{0}^{T} \|\tilde{\xi}_1(t)\|_2^2 + \|\tilde{u}(t)\|_2^2 dt \\
& \int_{0}^{T} \bigg( (1+K_3) M^2 e^{-\frac{2}{\epsilon}t}\| \tilde{\xi}(0)\|_2^2 \\&+ K_2K_3\tilde{\epsilon}^{2r}\big(\|\eta(0)\|_2^2 + \tilde{\epsilon}\|\tilde{\xi}(0)\|_2^2 \big) \bigg)dt \\
&\leq K_4 \bigg( \tilde{\epsilon}\|\tilde{\xi}(0)\|_2^2 + \|\eta(0)\|_2^2 \bigg),
\end{align*}
where in the last step we recall that we have chosen $T<\bar{T}$, where $\bar{T}>0$ is a fixed constant per the statement of the result, and we have chosen $K_4>0$ to be sufficiently large. 
\end{proof}

\subsection{Bounds on Small Time Horizons}
\begin{lemma}
Let Assumptions \ref{asm:square}-\ref{asm:growth} hold. Then for each $\bar{T}>0$ and each $\bar{T}>T$ and $\epsilon>0$ for each $(\xi,\eta) \in \R^n$ we have:
\begin{equation}
    a
\end{equation}
\end{lemma}

\subsection{Proof of Theorem \ref{thm:mpc}}

Let $u$ be such that $J_T(x_0,u) = V_T(x_0)$. Denote $\phi(\tau) = \phi(\tau,x_0,u)$ as the evolution of $x(t)$ for $\tau$ time units under control input $u$ starting from $x_0$. Consider $j \in [0,T-\Delta t]$. Then
\begin{align*}
    &V_T(x(\Delta t)) - V_T(x(0)) = V(\phi(\Delta t)) - \int_0^T l(\tau) \cdot d\tau & \\
    &\leq -\int_0^T l(\tau)  \cdot dt + \int_{\Delta t}^{T-j} l(\tau)\cdot d\tau \\ & + \min_{\tilde u} \int_{T-j}^{T+\Delta t} l(\phi(\tau,\phi(T-j),\tilde u),\tilde u(\tau))\cdot d\tau \\
    &\leq -\int_0^{\Delta t} l(\tau) \cdot d\tau + V_{j}(\phi(T-j)) \\ & \leq \bar \alpha(\sigma(\phi(T-j))) - \int_0^{\Delta t} l(\tau) \cdot d\tau
\end{align*}

As $V_T(\phi(0)) \geq \int_{0}^{T} l(t) dt$:
\begin{align*}
    W(\phi(T)) - W(\phi(0)) &\leq -k\int_{0}^{T} \| x(t)\|_2^2dt + \int_{0}^{T} l(t) dt \\
    &= V_T(\phi(0)) -k\int_{0}^{T} \| x(t)\|_2^2dt
\end{align*}

Noting that $0 \leq W(x) \leq \bar{\alpha}_W(\sigma(x))$ and $V_T(x) \leq \bar{\alpha}(\sigma(x))$, we can thus rearrange and bound terms to show the following:
\begin{align*}
    k\int_{0}^{T} \| x(t)\|_2^2dt \leq (\bar{\alpha}_W + \bar \alpha)\circ\sigma(\phi(0))
\end{align*}
Now consider $t^\ast \in [0,T]$ such that
\begin{equation*}
    t^\ast = \arg\min_{t\in [0,T]} \|x(t)\|_2^2
\end{equation*}
which exists by continuity of $x(t)$. Then we can note that
\begin{equation*}
    \|x(t^\ast)\|_2^2 \leq \frac{(\bar{\alpha}_W + \bar \alpha)\circ\sigma(\phi(0))}{kT}
\end{equation*}
Taking $j = T - t^\ast$ we have that
\begin{equation*}
    \|x(T-j)\|_2^2 \leq \frac{(\bar{\alpha}_W + \bar \alpha)\circ\sigma(\phi(0))}{kT}
\end{equation*}
We can combine this with the previous result on $V_T(x(\Delta t)) - V_T(x(0))$ to get the following:
\begin{align*}
    V_T(x(\Delta t)) - V_T(x(0)) &\leq -\int_0^{\Delta t} l(\tau) \cdot d\tau \\ &+ \bar \alpha(\frac{(\bar{\alpha}_W + \bar \alpha)\circ\sigma(\phi(0))}{kT})
\end{align*}
where we leverage the fact that $\bar \alpha$ is non-decreasing. 

Now note that
\begin{equation*}
    V_T(x(0)) = \int_{0}^{\Delta t} l(t) dt +  V_{T-\Delta t}(x(\Delta t))
\end{equation*}
Hence $\exists \bar T \geq 0$ s.t $\forall T \geq \bar T$
\begin{align*}
    V_T(x(\Delta t)) - V_{T-\Delta t} (x(\Delta t)) &= V_T(x(\Delta t)) - V_T(x_0) \\ &+ \int_0^{\Delta t} l(\tau) d\tau \\
    &\leq \bar \alpha(\frac{(\bar{\alpha}_W + \bar \alpha)\circ\sigma(\phi(0))}{kT})
\end{align*}
Also note that by assumption there exists $k_1,k_2$ s.t
\begin{align*}
    W(x) + V_{T-\Delta t}(x) &\leq W(x) + V_\infty(x) \\
    &\leq (k_1 + k_2)\|x\|^2
\end{align*}
Hence we can show the following
\begin{align*}
    \frac{d}{dt}(W(x) + V_{T-t}(x)) \leq -k \|x\|^2 \\
    \implies \ \frac{d}{dt}(W(x) + V_{T-t}(x)) \leq -\bar k (W(x) + V_{T-t}(x)) \\
    \implies \ W(x) + V_{T-t}(x) \leq e^{-\bar k t}(W(x(0)) + V_{T}(x(0)))
\end{align*}
where $\bar k = \frac{k}{k_1 + k_2}$. Thus we have the following:
\begin{align*}
    W(x(\Delta t)) + V_T(x(\Delta t)) &= W(x(\Delta t)) + V_{T-\Delta t}(x(\Delta t)) \\ &+ V_T(x(\Delta t)) - V_{T-\Delta t}(x(\Delta t)) \\
    &\leq e^{-\bar k \Delta t}(W(x(0)) + V_{T}(x(0))) \\ &+ \bar \alpha(\frac{(\bar{\alpha}_W + \bar \alpha)\circ\sigma(\phi(0))}{kT})
\end{align*}

Defining $Y = W + V_T$ and $\alpha = (\bar{\alpha}_w + \bar \alpha)$ completes the proof. Then, use the bound $\underbar{\alpha}_W\sigma(x)\leq W(x) \leq Y_T(x)$ we have 
\begin{equation}
    Y_T(\Phi(\Delta t)) \leq \bigg(e^{-\bar{k}\Delta t } + \bar \alpha(\frac{(\bar{\alpha}_W + \bar \alpha)}{\underbar{\alpha}_W kT})\bigg) Y_T(\phi(0)) 
\end{equation}

\subsection{Proof of Theorem \ref{thm:full_lin}}
To show global exponential stability, we note that it is sufficient to show that infinite horizon cost is bounded in the initial state and there is a Lyapunov function for the discrete time system that geometrically converges. On the first point, observe that we can use the conclusion of Lemma \ref{lemma:growth}, which applies to a more general class of systems. In particular, we can just ignore references to the zero dynamics $\eta$. We can apply similar reasoning to leverage the results of Theorem \ref{thm:mpc}, which gives us $Y_T$. Thus we have that $Y_T(\Phi(\Delta t)) - Y_T(\phi(0))  &\leq (e^{-\bar{k}\Delta t } + \bar \alpha(\frac{(\bar{\alpha}_W + \bar \alpha)}{\underbar{\alpha}_W kT}) - 1)Y_T(\phi(0))$.
Note that $\bar \alpha = \mathcal{O}(\epsilon)$ and $e^{-\bar{k}\Delta t} < 1$, so this can be made negative using sufficiently small $\epsilon$ for a given $\Delta t$ and $T$. This gives global exponential stability. \qedsymbol

% \begin{align*}
%     \epsilon C_1 \|\tilde \xi\|_2^2 \leq W^\epsilon(\tilde \xi) \leq \epsilon C_2 \|\tilde \xi\|_2^2 \\
%     \dot W(\tilde \xi, \tilde u) \leq (1-C)\|\tilde \xi\|_2^2 + \|\tilde u\|_2^2
% \end{align*}

\subsection{Proof of Theorem \ref{thm:full_lin}}
Consider $V_1(\tilde \xi) = \epsilon\tilde{\xi}^\top P \tilde \xi$ with the same $P,L,H$ as in Lemma \ref{lemma:min_phase_rate} and $V_2(\eta)$ from the converse Lyapunov theorem with constants as defined in Lemma $\ref{lemma:growth}$. Using an intermediate result from the aforementioned lemma, our bound on $V_\infty^\epsilon$, and noting that $\int_0^t \|\tilde \xi(\tau)\| \cdot d\tau \leq V_\infty^\epsilon$, we can say $\exists k_1 > 0$:
\begin{align*}
    V_2(\eta(t)) &\leq e^{-\tilde ct}V_2(\eta(0)) + \frac{1}{k}\int_0^t e^{-\tilde c(t-\tau)}\|\tilde \xi(\tau)\|\cdot d\tau \\
    &\leq e^{-\tilde ct}V_2(\eta(0)) + \mathcal{O}(\epsilon)\frac{\|\tilde \xi(0)\|^2_2 + \|\eta(0)\|^2_2}{k} \\
    V_2(\eta(t)) - V_2(\eta(0))&\leq (e^{-\tilde ct} - 1)V_2(\eta(0)) + \frac{R^2}{k}k_1 \epsilon
\end{align*}
By a similar approach in Lemma \ref{lemma:min_phase_rate}, we have that there exists a scaling $\alpha$ and $k_2 > 0$ s.t
\begin{align*}
    \dot{\tilde{V_1}}(\tilde \xi) = \alpha \dot V_1(\tilde \xi) &\leq -C\|\tilde \xi\|_2^2 + \|u\|_2^2 \\
    &\leq -\frac{b^\prime}{\epsilon}\tilde V_1(\tilde \xi) + \|u\|_2^2 \\
    \implies \tilde{V_1}(\tilde \xi) &\leq e^{-\frac{b^\prime}{\epsilon}t}\tilde V_1(\tilde \xi(0)) + \int_{0}^t e^{-\frac{b^\prime}{\epsilon}(t-\tau)}\|u(\tau)\|_2^2 \cdot d\tau \\
    &\leq e^{-\frac{b^\prime}{\epsilon}t}\tilde V_1(\tilde \xi(0)) + e^{-\frac{b^\prime}{\epsilon}t}\int_{0}^t e^{\frac{b^\prime}{\epsilon}\tau}\|u(\tau)\|_2^2 \cdot d\tau \\
    &\leq e^{-\frac{b^\prime}{\epsilon}t}\tilde V_1(\tilde \xi(0)) + O(\epsilon)R^2 e^{-\frac{b^\prime}{\epsilon}t}\frac{\mathcal{O}(\epsilon)}{b^\prime}[e^{\frac{b^\prime}{\epsilon}t} - 1] \\
    &\leq e^{-\frac{b^\prime}{\epsilon}t}\tilde V_1(\tilde \xi(0)) + k_2\epsilon^2 R^2
\end{align*}
where $b_1,b_2 > 0$ s.t $\epsilon b_1\|\tilde \xi\|_2^2 \leq V_1(\tilde \xi) \leq \epsilon b_2\|\tilde \xi\|_2^2$, and $b^\prime = Cb_2$. Choosing $\epsilon \leq \min\{\frac{\delta^2 k c_1}{k_1 R^2}, \frac{\delta^2 b_1 \alpha}{k_2 R^2}\}$ allows us to have exponential convergence of $(\tilde \xi, \eta)$ to the ball of radius $\delta$.

\subsection{Proof of Theorem \ref{thm:full_lin}}
Our proof will make use of the function
\begin{equation}
    W(\tilde{\xi},\eta) = V_1^\epsilon (\tilde{\xi})+ V_2^\epsilon(\eta)
\end{equation}
where $V_1^\epsilon(\tilde{\xi}) = \tilde{\xi}^T P \tilde{\xi}$ where $P$ is chosen so that $(F+LC)^TP + P(F +LC) = -2I$ where $F + LC$ is Hurwitz, and the function $V_2(\cdot)$ comes from a standard exponential stability converse theorem (see e.g. \cite{sastry2013nonlinear}) for the zero dynamics $\dot{\eta} = f_0(\eta)$. Namely, $V_2$ satisfies the following: 
\begin{align*}
    c_1 \| \eta\|_2^2\leq V_{2}(\eta) \leq c_2 \| \eta\|_2^2 \\
    \frac{d}{d\eta} V(\eta) f_0(\eta) \leq - c_3 \|\eta \|_2^2\\
    \| \frac{d}{d\eta} V_2(\eta)\|_2 \leq c_4\|\eta \|_2,
\end{align*}
for some positive constant $c_1,c_2,c_3,c_4>0$. 
\begin{align*}
    \dot{V}_1^{\tilde{\epsilon}}(\tilde{\xi}) &= \tilde{\xi}^T P \big [F + G[\tilde{\epsilon}^{r} \tilde{b}(\tilde{\xi},\eta)]+ \tilde{A}(\tilde{\xi},\eta)\tilde{u}  \big] \\
    & = \tilde{\xi}P[F + LC]\xi + \tilde{\xi} P[\tilde{\epsilon}^r\tilde{b}(\tilde{\xi},\eta) + \tilde{A}(\tilde{\xi},\eta)\tilde{u}]\\& - \tilde{\xi}^TPLC \tilde{\xi} \\
    &\leq -2 \|\tilde{\xi} \|_2^2 + \|P\|_2\| \tilde{\xi}\|C \big( \tilde{\epsilon}(\| \tilde{\xi}\|_2 + \| \eta\| )+ \|u\|\big)\\
    &+ \| L\| \|P\| \| \tilde{\xi}_1\|_2^2\\
    & \leq -(2- \tilde{\epsilon} \frac{3}{2}C \|P\| -\frac{1}{2}) \| \tilde{\xi}\|_2^2 + \tilde{\epsilon} \frac{1}{2}C \| P\| \| \eta\|_2^2 \\
    &+ \frac{1}{2}C^2 \|P \|^2 \| u\|_2^2 + \| L\| \|P\| \| \tilde{\xi}_1\|_2^2,
\end{align*}
here $C>0$ is as in Assumption \ref{asm:growth} and in the last step we have made repeated use of the inequality $a \cdot b < (a^2 + b^2)/2 $. Henceforth choosing $\tilde{\epsilon}$ to be small enough so that $\tilde{\epsilon} \frac{3}{2} \|P \| <\frac{1}{2}$, the preceding inequality can be reduced to
\begin{align}
    \dot{V}^\epsilon(\tilde{\xi})&\leq -\| \xi\|_2^2 + \tilde{C}_1 \big( \| \tilde{\xi}_1\|_2^2 + \epsilon \|\eta\|_2^2 +  \|u\|_2^2 \big) 
\end{align}
for some $\tilde{C}>1$ sufficiently large. 

Next let us consider:
\begin{align}
    \dot{V}_2(\eta) &= \frac{d}{d \eta} V_2(\eta)[f_0(\eta)+ g_0(\eta)\tilde{\xi}_1] \\
    &\leq -c_3\|\eta \|_2^2  +C c_4 \| \eta\|_2^2 \|\tilde{\xi}_1 \|_2^2 \\
    & \leq -(c_3 -\frac{1}{2})\|\eta\|_2^2 + C^2 c_4^2 \|\tilde{\xi}_1\|_2^2 \\
    & \leq -\frac{1}{c_2}V_2(\eta) + C^2 c_4^2 \|\tilde{\xi}_1 \|_2^2 \\
    &\leq -\tilde{C}_2 \|\eta\|_2^2 + \tilde{C}_3\|\tilde{\xi}_1\|_2
\end{align},
where $C>0$ is as in Assumption \ref{asm:growth}, and we have used in the second inequality $a\cdot b \leq (a^2 +b^2)/2$, and in the final inequality we have used $c_3 >2$ and chosen $\tilde{C}_2>0$ to be a sufficiently small constant, and $\tilde{C}_3>0$ to be sufficiently large.

\subsubsection{Full-state Linearizable} In the case where the system is full-state linearizable, we can simply ingorne the terms involving $\eta$ in the preceding expressions for $W$ and $\frac{d}{dt}{W}$. Rescaling $\hat{W}(\xi) = \frac{1}{\tilde{C}_1}$ we obtain: 
\begin{equation}
    \frac{\tilde{\epsilon}\lambda_{min}(P)}{\tilde{C}}\|\tilde{\xi}\|_2^2 \leq  W(\tilde{\xi}) \leq \frac{\tilde{\epsilon}\lambda_{max}(P)}{\tilde{C}} \|\tilde{\xi}\|_2^2 \\
\end{equation}
\begin{equation}
    \frac{d}{dt} \hat{W}(\tilde{\xi}) \leq -\frac{1}{\tilde{C}_1} \|\tilde{\xi}\|_2 + \|\tilde{\xi}_1\|_2^2 + \|u\|_2^2.
\end{equation}
Thus, if we choose $\sigma(\tilde{\xi}) = \|\tilde{\xi}\|_2^{2}$, let $\bar{\alpha}_V = \tilde{\epsilon}\hat{K}$ where $\hat{K}>0$ is as in Lemma \ref{lemma:growth}, let $\underline{\alpha}_{W} \frac{\tilde{\epsilon}\lambda_{min}(P)}{\tilde{C}}$, let  $\bar{\alpha}_{W} \frac{\tilde{\epsilon}\lambda_{max}(P)}{\tilde{C}}$ and $K_W = \frac{1}{\tilde{C}_1}$, then by the proof of Theorem \ref{thm:mpc} we have
\begin{equation}
 Y_T(\tilde(\Delta t)) \leq \bigg(e^{-\bar{k}\Delta t } + \bar \alpha(\frac{(\bar{\alpha}_W + \bar \alpha)}{\underbar{\alpha}_W kT})\bigg) Y_T(\tilde{\xi}(0))
 \end{equation}
 where $Y_T = \hat{W} + \tilde{V}_T^\tilde{\epsilon}$. If we have $T>\frac{\bar{\alpha}_V(\bar{\alpha}_V + \bar{\alpha}_W)}{K_W \underline{\alpha}_W (1-M(\Delta t))}$ then we will will have $Y_T(\tilde{\xi}_T(t_{k+1};\tilde{\xi_0})) < \rho Y_T(\tilde{\xi}_T(t_{k};\tilde{\xi_0}))$ for each $k \geq$, where $\tilde{\xi}_T(t_{k};\tilde{\xi_0})$ is the state trajectory generated by the RHC proccess from the initial condition $\tilde{\xi}_0$. This demonstrates that the RHC process decays geometrically between sampling instances, and thus converges to the origin exponentially. Note that for fixed $T\geq \Delta t >0$ this condition can be met by making $\tilde{\epsilon}$ sufficiently small.

\textbf{Step 1: Bounds on Optimal Trajectories:} To avoid notational clutter, in this portion of the proof we will simply let $(\tilde{\xi}(\cdot),\eta(\cdot))$ denote an optimal state trajectory and let $\tilde{u}(\cdot)$ denote an optimal control signal for the problem \eqref{eq:new_cost}. Ultimately, we will use the Lyapunov candidate
\begin{equation}
    W(\tilde{\xi},\eta) = V_1^\epsilon (\tilde{\xi})+ V_2^\epsilon(\eta)
\end{equation}
where $V_1^\epsilon(\tilde{\xi}) = \tilde{\xi}^T P \tilde{\xi}$ where $P$ is chosen so that $(F+LC)^TP + P(F +LC) = -2I$ where $F + LC$ is Hurwitz, and the function $V_2(\cdot)$ comes from a standard exponential stability converse theorem (see e.g. \cite{sastry2013nonlinear}) for the zero dynamics $\dot{\eta} = f_0(\eta)$. Namely, $V_2$ satisfies the following: 
\begin{align*}
    c_1 \| \eta\|_2^2\leq V_{2}(\eta) \leq c_2 \| \eta\|_2^2 \\
    \frac{d}{d\eta} V(\eta) f_0(\eta) \leq - c_3 \|\eta \|_2^2\\
    \| \frac{d}{d\eta} V_2(\eta)\|_2 \leq c_4\|\eta \|_2,
\end{align*}
for constants $c_1, c_2, c_3,c_4>0$ and without loss of generality we assume $c_3>2$ (if this is const the case then this condition can be satisfied by multiplying $V_2$ by a positive constant).

\begin{align}\
    V_2(\eta(t)) &\leq e^{-\frac{1}{c_3}t} V_2(\eta(0)) + \tilde{C}_1\int_{0}^t e^{-\frac{1}{c_3}t} \| \tilde{\xi}(t)\|_2^2 dt \\
    & \leq e^{-\frac{1}{c_3}t} V_2(\eta(0)) + \epsilon \tilde{C}_1 K_2\big( \| \tilde{\xi}(0)\|_2^2 + \|\eta(0)\|_2^2 \big), \\
    & =  \big( e^{-\frac{1}{c_3}t}+ \frac{\epsilon \tilde{C}_1 K_2}{c_1}\big)V_2(\eta(0)) + \epsilon \tilde{C}_1K_2 \| \xi(0)\|_2^2\label{eq:eta_bound}
\end{align}
where $K_1$ is the constant in Lemma \ref{lemma:growth} bounding the growth of the infinite horizon value function, and we have used the fact that $\int_{0}^T\|\tilde{\xi}(t) \|dt < \tilde{J}_{T}^\epsilon(\tilde{\xi}(0),\eta(0)) < \tilde{V}_{\infty}^\epsilon(\tilde{\xi}(0),\eta(0))$.

Note that the preceding equation demonstrates that for each $t \in \sp{0,\Delta t}$:
\begin{equation}
    \|\eta (t)\|_2^2 \leq \frac{3}{2c_1}\left(\|\tilde{\xi}(0) \|_2^2 +\| \eta(0)\|_2^2 \right),
\end{equation},
if we choose $\epsilon$ to be small enough so that $\epsilon \tilde{C}_1K_2 < \frac{1}{2}$. 

Next, consider the following bounds:
\begin{align*}
    \dot{V}^\epsilon(\tilde{\xi}) &= \tilde{\xi}^T P \big [F + G[\epsilon^{r} \tilde{b}(\tilde{\xi},\eta)]+ \tilde{A}(\tilde{\xi},\eta)\tilde{u}  \big] \\
    & = \tilde{\xi}P[F + LC]\xi + \tilde{\xi} P[\epsilon^r\tilde{b}(\tilde{\xi},\eta) + \tilde{A}(\tilde{\xi},\eta)\tilde{u}]\\& - \tilde{\xi}^TPLC \tilde{\xi} \\
    &\leq -2 \|\tilde{\xi} \|_2^2 + \| \tilde{\xi}\| \big(L_1 \epsilon(\| \tilde{\xi}\| + \| \eta\| )+ K\|u\|\big)\\
    &+ \| L\| \|P\| \| \tilde{\xi}_1\|_2^2\\
    & \leq -(2- \epsilon \frac{3}{2}L_1 \|P\| -\frac{1}{2}) \| \tilde{\xi}\|_2^2 + \epsilon \frac{1}{2}L_1 \| P\| \| \eta\|_2^2 \\
    &+ \frac{1}{2}K^2 \|P \|^2 \| u\|_1^2 + \| L\| \|P\| \| \tilde{\xi}_1\|_2^2,
\end{align*}
where $L_1,K>0$ are as in Assumption \ref{asm:growth} and in the last step we have made repeated use of the inequality $a \cdot b < (a^2 + b^2)/2 $. Henceforth choosing $\epsilon$ to be small enough so that $\epsilon \frac{3}{2} \|P \| <\frac{1}{2}$, the preceding inquality can be reduced to
\begin{align}
    \dot{V}^\epsilon(\tilde{\xi})&\leq -\| \xi\|_2^2 + \tilde{C} \big( \| \tilde{\xi}_1\|_2^2 + \epsilon \|\eta\|_2^2 +  \|u\|_2^2 \big) 
\end{align}
for some $\tilde{C}>1$ sufficiently large. 
Now, consider the composite function:
\begin{equation}
    \mathcal{V}^\epsilon(\tilde{\xi},\eta,t) = \alpha V_1^\epsilon(\tilde{\xi}) + V_{T-t}^\epsilon(\tilde{\xi}, \eta),
\end{equation}
whose time derivative is bounded by:
\begin{align}
    \dot{\mathcal{V}}(\tilde{\xi},\eta,t) &\leq -\alpha \|\xi\|+ \epsilon  \|\eta\|\\
    &\leq -\alpha (\|\xi\| + \epsilon \|\eta\|)+ 2\epsilon\|\eta\|_2^2
\end{align},
where we have used the fact that $\alpha <2$. 
Next, note that 
\begin{equation}\label{eq:growth2}
\tilde{c}_1 \epsilon \| \tilde{\xi}\|_2^2\leq \mathcal{V}(\tilde{\xi}) \leq \tilde{c}_2 (\epsilon\|\tilde{\xi}\|_2^2 + \epsilon^2\|\eta\|_2^2)
\end{equation}
where
\begin{equation}
    \tilde{c}_1 = \alpha \lambda_{min}(P), \ \ \ \tilde{c}_2 = K_1 + \alpha \lambda_{max}(P),
\end{equation}
where the constant $K_1>0$ is from the bound on $V_\infty^\epsilon$ in Lemma \ref{lemma:growth}. Thus, we have:
\begin{equation}
    \dot{\mathcal{V}}(\tilde{\xi},\eta,t) = -\frac{\alpha}{\epsilon \tilde{c}_1} \mathcal{V}(\tilde{\xi},\eta,t) + 2\epsilon \| \eta\|_2^2,
\end{equation}
which, by the comparison principle, yields: 
\begin{align}
    \mathcal{V}(\tilde{\xi},\eta,t) \leq e^{-\frac{\alpha}{\epsilon \tilde{c}_2} t} + 2\epsilon \int_{0}^{t} e^{-\frac{\alpha}{\epsilon \tilde{c}_2} t} +\mathcal{V}(\tilde{\xi},\eta,0) \|\eta(t) \|_2^2 dt.
\end{align}
By further choosing $\epsilon$ to be small enough so that \twnote{todo} holds, the preceding bound gives us:
\begin{align}
    \mathcal{V}(\tilde{\xi},\eta,t) &\leq   e^{-\frac{\alpha}{2 \tilde{c}_1\epsilon}t} \mathcal{V}(\tilde{\xi},\eta,0) \\
    & + \epsilon \frac{3}{ c_1} \left(\| \tilde{\xi}(0)\|_2^2 + \|\eta(0)\|_2^2 \right) \int_{0}^{t} e^{-\frac{\alpha}{\epsilon \tilde{c}_2} t} dt\\
    &\leq 
    e^{-\frac{\alpha}{2 \tilde{c}_2 \epsilon}t} \mathcal{V}(\tilde{\xi},\eta,0) + \frac{3 \epsilon^2}{2 \alpha c_2}\left(\| \tilde{\xi}(0)\|_2^2 + \| \eta(0)\|_2^2\right).
\end{align}
Next, if we choose
$\epsilon$ to be small enough so that $-\epsilon\frac{2 \tilde{c}_2}{\alpha} \ln{\epsilon} <\Delta t$ then from the preceding bound and \eqref{eq:growth2} we can obtain:
\begin{equation}
    \|\xi(\Delta t)\|_2^2 \leq \epsilon \tilde{C}_2 \left(\| \tilde{\xi}(0)\|_2^2 + \| \eta(0)\|_2^2 \right),
\end{equation}
where $\tilde{C}_2>0$ is chosen to be sufficiently large. We can then transform this into abound of the form:
\begin{equation}
V_1^\epsilon(\tilde{\xi}(\Delta t)) \leq \epsilon \tilde{C}_3 \left( V_1^\epsilon(\tilde{\xi}(0)) + V_2(\eta(0)) \right)
\end{equation}
where $\tilde{C}_3>0$ is once again a sufficiently large constant. Moreover, if we choose $\epsilon$ to be small enough so that $\frac{\epsilon \tilde{C}_1K_1}{c_1} < 1 - e^{-\frac{1}{c_3}\Delta t}$ then using equation \eqref{eq:eta_bound} and the bounds on $V_2$ in \twote{todo} we can bounds
\begin{equation}
    V_2(\eta(\Delta t)) \leq \rho V_2(\eta(0)) + \tilde{C}_4V_1^\epsilon(\tilde{\xi}(0))
\end{equation}
for some $\tilde{C}_4>0$ sufficiently large and $0<\rho <1$.

\textbf{Proof of Stability}

\begin{align}
    V_1(\eta) &= \nabla V_2(\eta)[f_0(\eta) + g_0(\eta) \tilde{\xi}_1]\\
    &\geq -L_3 c_4 \|\eta\|_2^2 - K c_4 \|\tilde{\xi} \| \\
    &\geq  -(\frac{L_3c_4}{\tilde{c}_3}+\frac{1}{2}K^2c_4^2)V_2(\eta) - \frac{1}{2}\| \xi\|_2^2 \\
    &\geq - \tilde{C}_5 V_2(\eta) - \frac{1}{2} \| \tilde{\xi}\|_2^2
\end{align}
\begin{align}
    V_2(\eta(\Delta t)) &\geq e^{-\tilde{C}_5 \Delta t} V_2(\eta) - \frac{1}{2} \int_{0}^{\Delta t} e^{-\tilde{C}_5 \Delta t}\| \tilde{\xi}(t)\|_2^2dt \\
    &\geq e^{-\tilde{C}_5 \Delta t} V_2(\eta) - \frac{1}{2} K_1(\epsilon \|\tilde{\xi}(0)\| + \epsilon^2\|\eta(0) \|_2^2 )
\end{align}

\begin{equation}
    V_1^{\epsilon}(\tilde{\xi}_k)\leq \tilde{\rho}^{k} V_1^\epsilon(\tilde{\xi}_0) + \sum_{j=0}^{k-1} \tilde{\rho}^{k-j-1}V_2(\tilde{\xi}_j)
\end{equation}
\begin{equation}
    V_2^\epsilon(\tilde{\xi}_k) \leq \rho^{k} + \tilde{C}_4\sum_{j=0}^{k-1} \rho^{k-j-1} V_1^\epsilon(\xi_k)
\end{equation}

\subsection{Proof of Theorem \twnote{todo}.}

Throughout the proof, to simplify the arguments, we will restrict our attention to the case where $1>T\geq \Delta t >0$. Given this restriction, we seek an upper-bound on $\tilde{V}_T(\tilde{\xi}(0),\tilde{\eta}(0))$. Two will be required for our subsequent arguments. 

\textbf{Upper-bounds on $\tilde{V}_T$:} 
\begin{align}
    \frac{d}{dt} \| \bar{x}(t)\|_2^2 &= \bar{x}(t)^T[\bar{F}(\bar{x}) +\bar{G}(\bar{x}(t))u(t)] \\
    &\leq L_F \|x(t)\|_2^2 + L_G\| x(t)\|_2\| u(t)\|_2 \\
    &\leq (L_F +\frac{1}{2}L_G^2)\|x(t)\|_2^2 + \frac{1}{2} L_G^2 \|u(t)\|_2^2
\end{align}

From this we obtain:
\begin{align}\label{eq:x_bound1}
    \|\bar{x}(t)\|_2^2 &\leq e^{(L_F + \frac{1}{2}L_G^2)t} \|\bar{x}(t)\|_2^2 \\
    &+ \frac{1}{2}L_G^2\int_{0}^{T}  \|u(t)\|_2^2 e^{(L_F + \frac{1}{2}L_G^2)(t-\tau)}\| u(\tau)\|d\tau \\
    &\leq \bar{C}_1\left(\|x(0)\| + \int_{0}^{t}\|u(\tau)\| d \tau \right)  \label{eq:state_timebound}
\end{align}
where $\bar{C}_1$ is a sufficiently large constant and in obtaining the second inequality we have used $t<T\leq1$, so that the preceding inequality holds for all choices of time horizon.

First we upper bound $\tilde{V}_T$ as a function of the prediction horizon $T>0$. In particular, suppose we apply the control $\bar{u}_1(\cdot) \equiv 0$. Using the preceding bound on $\|\bar{x}(t)\|_2^2$ We may bound the value function as follows: 
\begin{equation}\label{eq:time_bound}
    \tilde{V}_T(\bar{x}(0)) \leq \tilde{J}_T(\bar{u}_1(\cdot),\bar{x}(0)) < \bar{C}_1T \|\bar{x}(0)\|_2^2.
\end{equation}
Note that this bound depends on $T$ but not $\epsilon$.

Next, consider the control signal defined by $\bar{u}_2(t)= \tilde{A}^{-1}(\tilde{\xi}(t),\eta(t))[-\tilde{b}(\tilde{\xi}(t),\eta(t)) + K\tilde{\xi}(t)]$ where $K$ is chosen so that $F+GK$ is Hurwitz and chosen so that for some $M>0$ we have $\tilde{\xi}(t) \leq Me^{-\frac{t}{\epsilon}}\|\tilde{\xi}(t)\|$. Next we seek to bound the growth of the zeros under the application of this control law. 

\begin{align}
\frac{d}{dt} (\| \eta(t)\|_2^2 )&= 2 \eta(t)^T[f_0(\eta) + g(\eta)\tilde{\xi}] \\
& \leq 2 L_F\|\eta(t)\|_2^2 + 2K\|\eta(t) \|_2\|\tilde{\xi}(t) \|_2 \\
&\leq 2(L_f + L_F^2)\|\eta(t)\|_2^2 + \| \tilde{\xi}(t)\|_2^2 \\
\end{align}
which by the comparison principle yields:
\begin{align}
\|\eta(t) \|_2^2 &\leq e^{2(L_f + L_F^2)t}\| \eta(0)\| + \int_{0}^{t}  e^{2(L_f + L_F^2)(t-\tau)}\|\tilde{\xi}(\tau)\|_2^2 d\tau \\
&\leq e^{2(L_f + L_F^2)t}\| \eta(0)\| \\
&+ \int_{0}^{t}  e^{2(L_f + L_F^2)(t-\tau)}Me^{-\frac{1}{\epsilon}\tau}\|\tilde{\xi}(0)\|_2^2 d\tau \\
&\leq \bar{C}_2(\|\eta(0)\|_2^2 + \epsilon \| \xi(0)\|),
\end{align}
where $\bar{C}_2>0$ is chosen to be sufficiently large. 
Combining the preceding inequalities yields an inequality of the form:
\begin{equation}
    \|\bar{u}_2(t)\|_2^2 \leq \bar{C}_3 \left( \|\tilde{\xi}(0)\|_2^2 +  \|\eta(0)\|_2^2\right) 
\end{equation}
for some $\bar{C}_3>0$ sufficiently large.

\begin{align}
    \tilde{V}_T(\tilde{\xi}(0),\eta(0)) &\leq \tilde{J}_T(\bar{u}_2(\cdot);\tilde{\xi}(t),\eta(t))\\
    &\leq \int_{0}^{T}Me^{-\frac{2}{\epsilon}} \|\tilde{\xi}(0)\|_2^2 + \epsilon^{2}\big(\|\tilde{\xi}(0)\|_2^2 + \|\eta(0)\|_2^2 \big) \\
    & \leq \tilde{C}_4 \big(\epsilon \|\tilde{\xi}(0)\|_2^2 + \epsilon^2\|\eta(0)\|_2^2 \big), \label{eq:nmp_finite}
\end{align}
where we have again used the fact that $T<1$ and $\bar{C}_4$ is a sufficiently large constant. Note that this bound depends on $\epilon$ but not $T$.

\textbf{Instability Bounds:}

\textit{Part 1:} First we demonstrate that there exists $\epsilon^*>0$ sufficiently small so that for each $0<\epsilon<\epsilon^*$ and $0< \Delta t = T \leq 0$ the   resulting receding horizon controller will fail to stabilize the zero dynamics. Since the zero dynamics $\dot{\eta}= f_0(\eta)$ are exponentially unstable, the time reversed dynamics $\dot{\eta} =-f_0(\eta)$ must be exponentially stable and thus there must exist a Lyapunov function $V_2$ which satisfies: 
\begin{align*}
    \hat{c}_1 \| \eta\|_2^2\leq V_{2}(\eta) \leq \hat{c}_2 \| \eta\|_2^2 \\
    -\frac{d}{d\eta} V(\eta) f_0(\eta) \leq - \hat{c}_3 \|\eta \|_2^2\\
    \| \frac{d}{d\eta} V_2(\eta)\|_2 \leq \hat{c}_4\|\eta \|_2,
\end{align*}

\begin{align}
    \dot{\hat{V}}_2(\eta)&= \frac{d}{d\eta}V_2(\eta)[f_0(\eta) + g_0(\eta)\tilde{\xi}] \\
    & \geq \hat{c}_3\| \eta\|_2^2 +C \hat{c}_4\|\eta\|_2\|\tilde{\xi}_1\|_2 \\
    &\geq \bar{C}_5 \hat{V}_2(\eta) - {C}_6\|\tilde{\xi}(t)\|_2^2 
\end{align}
for appropriately chosen constants $\bar{C}_5,\bar{C}_6>0$. Applying the comparison principle yields
\begin{align}
\hat{V}_2(\eta(T)) &\geq e^{\bar{C}_5T} \|V_2(\eta)\|_2^2 - \bar{C}_6 \int_{0}^{T} e^{\bar{C}_5(T-t)}\|\tilde{\xi}(t)\|_2^2 dt \\
&\geq e^{\bar{C}_5T}V_2(\eta)_2^ - \bar{C}_7\left(\epsilon\|\tilde{x}(0)\|_2^2 +\epsilon^2 \|\eta(0) \|_2^2 \right)
\end{align}
where we have used the second upper-bound for the non-minimum-phase case in \eqref{eq:nmp_finite}. Thus, there exists a constant $\bar{C}_8>1$ sufficiently such that for each $\epsilon>0$ sufficiently small we have:
\begin{equation}
   \hat{V}_2(\eta(T)) \geq
\bar{C}_8 V_2(\eta(0))- \bar{C}_{7} V_1^\epsilon(\tilde{\xi}(0)),
\end{equation}
where $V_1^\epsilon$ is as in the proof of Lemma \twnote{todo}.  Note, that if $\bar{C}_8 V_1(\tilde{\xi}(0)) \leq \bar{C}_8  V_2(\eta(0))$ then we will have $\hat{V}_2(\eta(T)) > \hat{V}_2(\eta(0))$. This will be our basis for demonstrating that the closed-loop system is unstable for $\epsilon$ sufficiently small. 

Next, we claim that there exists $\bar{
C}_8>0$ sufficiently large such that for each $\epsilon>0$ sufficiently small we have:
\begin{equation}
    V_1^\epsilon(\tilde{\xi}(T)) \leq \epsilon \bar{C}_9 \big( V_1^\epsilon(\tilde{\xi}(0)) + \hat{V}_2(\eta(0))\big).
\end{equation}
In particular, a bound of this form can be derived by following the steps used to derive the bound \eqref{eq:xi_decay1}, except the upper-bound on $V^\epsilon_T$ in \eqref{eq:nmp_finite} is used in place of the upper-bound use for the minimum-phase case. 

Next, let $\{(\tilde{\xi}^{k},\eta^k)\}_{k=0}^{\infty}$ be the sequence of iterates generated at the sampling instances of the RHC scheme with $T=\Delta t$ and $\tilde{\xi}^0 = 0$ and $\eta^0>0$.  
\begin{equation}
    \hat{V}_2(\eta_1)> \bar{C}_8\hat{V}_2(\eta^0)
\end{equation}
\begin{equation}
    V_1^\epsilon(\tilde{\xi}^1) \leq \epsilon \bar{C}_9 \hat{V}_2(\eta^0) \leq \epsilon \bar{C}_9 \bar{C}_8\hat{V}(\eta^0).
\end{equation}
More generally, if we assume that
\begin{equation}
V_1^{\epsilon}(\tilde{\xi}^k)\label{eq:ratio} <\frac{C_8}{\bar{C}_9} \hat{V}_{2}(\eta^k)
\end{equation}
then we will have
\begin{equation}\label{eq:zero_go_boom}
\hat{V}_2(\eta^{k+1})> \hat{V}_2(\eta^{k}).
\end{equation}
Moreover, under this hypothesis, for $\epsilon >0$ sufficiently small we will have
\begin{equation}
    V_1^{\epsilon}(\tilde{\xi}^{k+1}) \leq  \frac{\bar{C}_8}{\bar{C}_9}\hat{V}_2(\eta^{k+1}).
\end{equation}
Since \eqref{eq:ratio} for $k=0$, it will also hold for all iterates $k>0$ for $\epsilon$ sufficiently small. Thus, for $\epsilon$ sufficiently small \eqref{eq:zero_go_boom} will hold for each $k$, indicating that the zeros escape to infinity and that the RHC process fails to stabilize the system.

\textit{Part 2}: Next, letting $\bar{\epsilon}$ be small enough so that the RHC process fails to stabilize the zeros, as above, our goal is to demonstrate that there exists $1>T^*>0$ sufficiently small that for each $T>T^*$ the RHC process does not stabilize the system.  Similar to before, since the natural dynamics $\dot{\bar{x}} = \bar{F}(\bar{x})$ are exponentially unstable, there must exists constants $\bar{c}_1,\bar{c}_2,\bar{c}_3,\bar{c}_4$ such that:
\begin{align*}
    \bar{c}_1 \| \eta\|_2^2\leq V_{2}(\eta) \leq \bar{c}_2 \| \eta\|_2^2 \\
    -\frac{d}{d\eta} V(\eta) f_0(\eta) \leq - \hat{c}_3 \|\eta \|_2^2\\
    \| \frac{d}{d\eta} V_2(\eta)\|_2 \leq \hat{c}_4\|\eta \|_2,
\end{align*}

\begin{align}
    \dot{\bar{V}}(\bar{x}) &\geq \frac{d}{d\bar{x}} \bar{V}(\bar{x})[\bar{F}(\bar{x}) + \bar{G}(\bar{x})u] \\
    &\geq \bar{c}_3 \|\bar{x}\|_2^2 - \bar{c}_4K \| \bar{x}\| \|u\| \\
    & \geq \frac{\bar{c}_3}{2}\|\bar{x}\|_2^2 - \frac{2\bar{c}_4K}{\bar{c_3}}u \\
    &\geq \bar{C}_9 \|\bar{x}\|_2^2 - \bar{C}_{10} \|u\|_2^2
\end{align}
The preceding equation demonstrates that if $\bar{C}_6\|u(t)\|_2^2 < \bar{C}_5\|\bar{x}(t)\|_2^2$ for each $t \in \sp{0,T}$, then $\bar{V}$ will be strictly increasing when $\bar{x} \neq 0$, which will immediately demonstrates that the MPC process does not stabilize the system. Towards this end, for each $\epsilon > \bar{\epsilon}$ we can upperbound the growth of the state trajectory as follows using \eqref{eq:time_bound}:
\begin{equation}
\int_{0}^T \|u(t)\|_2^2 \leq
\frac{1}{\bar{\epsilon}^2} \bar{V}_T^\epsilon(\bar{x}(0)) \leq \frac{1}{\bar{\epsilon}^2} \bar{C}_1 T\|\bar{x}(0)\|_2^2
\end{equation}
Then plugging this into \eqref{eq:state_timebound}
\begin{align}
    \|\bar{x}(t)\|_2^2 &\leq \bar{C}_1(\|x(0)\|_2^2 + \frac{1}{\bar{\epsilon}^2} \bar{C}_1 T\|\bar{x}(0)\|_2^2) \\
    &\leq \bar{C}_{11}\|\bar{x}(0)\|_2^2
\end{align}

Then, the minimum principle dictates that 
\begin{equation}
    u(t) = -\frac{1}{2}\bar{G}(\bar{x})^{T} p(t),
\end{equation}
where the costate $p \colon \sp{0,T} \to \R^n$ satisfies the terminal boundary value problem: 
\begin{equation}
\dot{p}(t) &= \underbrace{-\frac{d}{dx}F^*(\bar{x}(t),p(t))^Tp(t) - \tilde{\xi}(t)}_{M(t,p(t))} \ \ p(t) =0
\end{equation}
where 
\begin{equation*}
    F^*(\bar{x}^*(t), p^*(t)) = \bar{F}(\bar{x}^*(t)) - \bar{G}(\bar{x}^*(t))\bar{G}(\bar{x}^*(t))^Tp^*(t).
\end{equation*}

\begin{align}
    \frac{d}{dt} \| p(t)\|_2^2 &= p(t)^T[-\frac{d}{dx}\bar{F}(\bar{x}^*(t))^Tp(t) -  \tilde{\xi}^*(t)] \\ 
    & \leq L_F\|p(t)\|^2 \| x(t)\| + \|x(t) \|_2 \| p(t)\|_2 \\
    & \leq \bar{C}_7 \big( (\|p(t)\|_2^2)^2 + \| p(t)\|_2^2 + \|\bar{x}(t)\| \big)
\end{align}
\begin{equation}
    \|p(t)\|_2^2 \leq \bar{C}_{13}\|x(0)\| + \bar{C}_{12}\int_{0}^{T} \|p(t)\|_2^2 + (\| p(t)\|_2^2)^T dt
\end{equation}
 Then, by the comparison principle, if we set $\delta = \bar{C}_{13}\| x(0)\|_2^2$ for each $\epsilon>\bar{\epsilon}$ we will have $\| p(t)\|_2^2 \leq a^{\delta}(t)$, where $\delta = \bar{C}_{13}\|x(0) \|$ and $a^{\delta}(\cdot)$ denotes the maximal solution to the Riccatti-type equation:
\begin{equation}
    \dot{a}^{\delta}(t) = \delta + \bar{C}_{12}a^{\delta}(t) + \bar{C}_{12}(a^{\delta}(t))^{2}, \ \ a(t) =0.
\end{equation}

In general, this differential equation my not be defined on the whole interval $\sp{0,T}$, as Riccati odes of this type are wellknown to escape to infinity in finite time. However, let us restrict ourselves to the initial conditions such that  $\delta=\bar{C}_{13}\| x(0)\|_2^2 \leq \bar{\delta}$ for some constant $\bar{\delta}>0$ which will be specified later. Clearly there exists exists $\bar{T}>0$ such that for each $t<\bar{T}$ we have $a^{\bar{\delta}}(t)<1$. Moreover, by inspection, we also have $0 \leq a^{\delta}(t)\leq a^{\bar{\delta}}(t) <1$ for each $\sp{0,\bar{T}}$. Thus, on the interval $\sp{0,\bar{T}}$ for each $\delta <\bar{\delta}$ we clearly have:
\begin{equation}
  \dot{a}^{\delta} \leq \delta + 2\bar{C}_{12} a(t).
\end{equation}
Thus, we have:
\begin{align}
    a^\delta(t) &\leq \delta \int_{0}^{t}e^{2\bar{C}_{12}(t-\tau)}  d\tau \\
    & \leq \delta \bar{C}_{13}t 
\end{align}
Together the preceding arguments imply:
\begin{equation}
    \|p(t)\|_2^{2} \leq \bar{C}_{14} T\|\bar{x}(0)\|_2^2
\end{equation}
if $T \leq \bar{T}$ and $\delta \leq \bar{\delta}$.

For fixed coefficient $\delta, \bar{C}_{12}$ there exists $1\geq\bar{T}>0$ such that $a(\cdot)$ has a well defined solution on $\sp{0,\bar{T}}$. Then letting

we will have for each $\bar{T}>T>0$
\begin{equation}
    \| p(t)\|_2^2 \leq \bar{C}_{15}t \leq \bar{C}_{15}T, 
\end{equation}.
This in turn lets us bound
\begin{equation}
    \|u(t)\|_2^2 \leq  \bar{C}_{16}\|\bar{x}()\| T
\end{equation}
for some $\bar{C}_{16}>0$ sufficiently large.
