# Supplementary material for: On the Computational Consequences of Cost Function Design in Nonlinear Optimal Control
Source: arXiv:2204.01986 source file (2022-11-18)
Supplement: Supplementary file 2 [file appendix.tex]

\subsection{Auxilary Lemmas}

\begin{lemma}\label{lemma:growth}
Let Assumptions \ref{asm:relative_degree},\ref{asm:strict_fb}, and \ref{asm:growth} hold. Also assume that $\dot \eta = f_0(\eta)$ is globally exponentially stable. Then there exist $K_1>0$ such that for each $0<\epsilon \leq 1$ the infinite horizon performance satisfies $V_\infty^\epsilon(x) \leq K_1\big(\epsilon\|\tilde{\xi}_2^2\| + \epsilon^{2(r+1)} \|\eta\|_2^2\big)$.
\end{lemma}

\begin{lemma} \label{lemma:min_phase_rate}
Let the assumptions in Lemma \ref{lemma:growth} hold. Then there exists constants $C_1, C_2,C_3>0$ and such that for each $\epsilon>0$ sufficiently small there exists a continuously differentiable function $W^\epsilon \colon \R^n \to \R^n$ which satisfies for each $(\tilde{\xi},\eta) \in \R^n$ and $u \in \R^q$:
\begin{equation}
    C_1\big(\epsilon\|\tilde{\xi}\|_2^2+ \|\eta\|_2^2\big)\leq W^\epsilon(\tilde{\xi},\eta) \leq C_2\big(\epsilon\| \tilde{\xi}\|+ \|\eta\|_2^2\big) 
\end{equation}
\begin{equation}
    \dot{W}(\tilde{\xi}, \eta,\tilde{u}) \leq -C\big(\| \tilde{\xi}\|_{2}^2 + \|\eta\|_2^2 \big)+ \|\tilde{\xi}_1 \|_2^2 + \|\tilde{u}\|_2^{2}
\end{equation}
\end{lemma}

\subsection{Proof of Theorem \ref{thm:min_phase}}
To show global exponential stability, we note that it is sufficient to show that infinite horizon cost is bounded in the initial state and there is a Lyapunov function for the discrete time system that geometrically converges. On the first point, observe that we can use the conclusion of Lemma \ref{lemma:growth}, which applies to a more general class of systems. In particular, we can just ignore references to the zero dynamics $\eta$. We can apply similar reasoning to leverage the results of Theorem \ref{thm:mpc}, which gives us $Y_T$. Thus we have that $Y_T(\Phi(\Delta t)) - Y_T(\phi(0))  &\leq (e^{-\bar{k}\Delta t } + \bar \alpha(\frac{(\bar{\alpha}_W + \bar \alpha)}{\underbar{\alpha}_W kT}) - 1)Y_T(\phi(0))$.
Note that $\bar \alpha = \mathcal{O}(\epsilon)$ and $e^{-\bar{k}\Delta t} < 1$, so this can be made negative using sufficiently small $\epsilon$ for a given $\Delta t$ and $T$. This gives global exponential stability. \qedsymbol
